# Supplementary material for: Noncommutative Geometry and Quantum Group Symmetries
Source: arXiv:0811.3187 source file (2008-11-19)
Supplement: Supplementary file 1 [file supp-pdf.tex]

%% arXiv admin created this file as workaround since we don't support eTex 
%% at this time.
\endinput
